# Supplementary material for: SpectAcLE: An Improved Method for Modeling Light Echo Spectra
Source: arXiv:2310.01501 source file (2023-10-02)
Supplement: Supplementary file 1 [file 04Effective_PSF.tex]

\section{Effective PSF}
\label{sec:eff_PSF}
\noindent {\bf Effective PSF:} In general, the PSF of an observation is measured in terms of the Full-Width-Half-Maximum (FWHM). For our purposes, the PSF usually can be sufficiently characterized with a circular Gaussian having a single width $\sigma_{\rm PSF}$, as measured by standard PSF photometry.
% The $\sigma_{PSF}$ of that Gaussian can be calculated as \redpen{FILL ME: equation}. % RP: what do you mean calculate sigma_PSF? It's measured by photometry on the image
We denote the angle between the the light echo profile box $A_{\rm box}$ and the line perpendicular to the ``crest'' of the light echo $A_{\rm LE}$ (maximum projection scale) as $\alpha$, such that $\alpha=0$ when the profile box is perpendicular to the crest ($A_{0,{\rm box}}=A_{\rm LE}$). Then $\sigma_{\rm PSF,eff}$ is related to $\sigma_{\rm PSF}$ with the following relation:

\begin{eqnarray}
\sigma_{\rm PSF,eff}  =  \frac{\sigma_{\rm PSF}}{\cos{\alpha}} \label{eq:PSF_eff}
\end{eqnarray}
 
We note that for small angles of $\alpha$, $\sigma_{\rm PSF,eff} \approx \sigma_{\rm PSF}$. This is not a big effect, and needs to be taken into account only for $\alpha\gtrsim15\deg$ (see Figure~\ref{fig:eff_psf}).
This means that for cases with large $\alpha$, we must estimate the position angle of the ellipsoid-dust intersection arclet $A_{\rm LE}$ in order to get $\sigma_{\rm PSF,eff}$ (see step 2 in Section~\ref{sec:mthd_proc}).
\\\\

\begin{figure}
\epsscale{1.0}
\includegraphics[width=\linewidth]{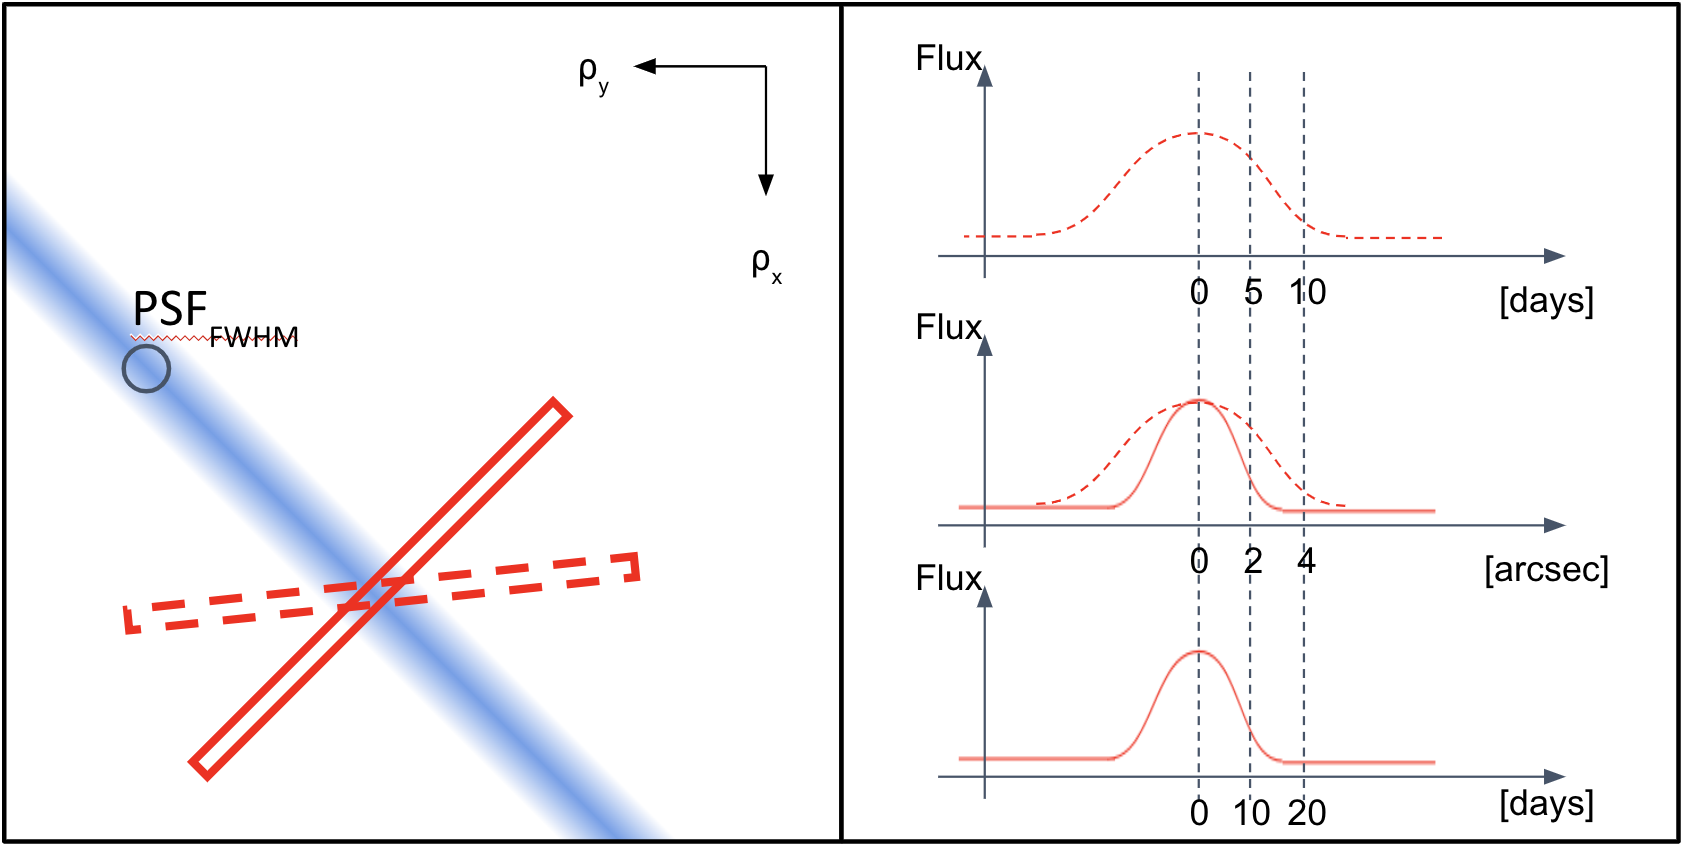}
\figcaption{Effect of position angle on effective PSF. For a given PSF (in this case a circular one for simplicity), it's effective width on the light echo profile will be wider for shallower angles in respect to $A_{LE}$ (see \ref{fig:prinicipalaxes}). \label{fig:eff_psf}}
\end{figure}
